# Supplementary material for: DUAL-GLOW: Conditional Flow-Based Generative Model for Modality Transfer
Source: arXiv:1908.08074 source file (2019-08-21)
Supplement: Supplementary file 1 [file expfig-supp.tex]

%%% suvr
\begin{figure}[]
	\centering
	\includegraphics[width=0.98\columnwidth]{./figs/suvr.eps}
	\caption{\label{fig:suvr} The relative SUVRs for 16 ROIs. }
\end{figure}

%%% mae
\begin{figure}[]
	\includegraphics[width=0.98\columnwidth]{./figs/corr.pdf}
	\caption{\label{fig:exp2} Mean absolute error on held out test set generations, stratified by age, sex, and disease status.}
\end{figure}

%%%%%%%%%%%%%%%%%%%%%%%%%%%%%%%%%%%%%%% demogra %%%%%%%%%%%%%%%%%%%%%%%%%%%
%\begin{figure}[]
%	\centering
%	\begin{subfigure}{7.5cm}
%		\centering\includegraphics[width=7.5cm]{./figs/demogra-1.png}
%	\end{subfigure}
%	\begin{subfigure}{5.5cm}
%		\centering\includegraphics[width=5.5cm]{./figs/demogra-2.png}
%	\end{subfigure}
%	\caption{\label{fig:demographics} Demographics of all individuals included in our experiments. All information was collected from metadata provided by ADNI.}
%\end{figure}

%%%%%%%%%%%%%%%%%%%%%%%%%%%%%%%%% samples %%%%%%%%%%%%%%%%%%%%%%%%%%%%%%
%%%% ADs
\begin{figure*}[]
	\centering
	\begin{tabular}{ccc|ccc}
		MRI & GT & Synthetic & MRI & GT & Synthetic \\
		
		%%%%%%%%%%%%%%  s
		\begin{subfigure}{2.cm}
			\centering\includegraphics[width=2.cm]{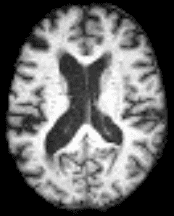}
		\end{subfigure}&
	\begin{subfigure}{2.cm}
		\centering\includegraphics[width=2.cm]{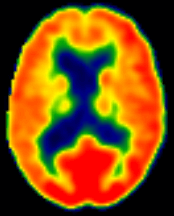}
	\end{subfigure}&
\begin{subfigure}{2.cm}
	\centering\includegraphics[width=2.cm]{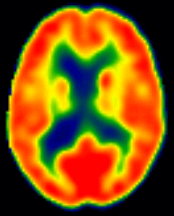}
\end{subfigure}&

	\begin{subfigure}{2.cm}
	\centering\includegraphics[width=2.cm]{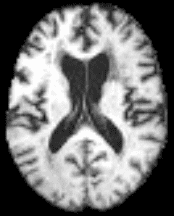}
\end{subfigure}&
\begin{subfigure}{2.cm}
	\centering\includegraphics[width=2.cm]{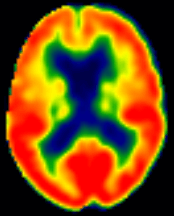}
\end{subfigure}&
\begin{subfigure}{2.cm}
	\centering\includegraphics[width=2.cm]{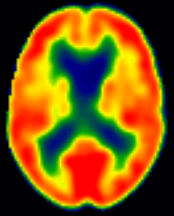}
\end{subfigure} \\

		%%%%%%%%%%%%%%  a
			\begin{subfigure}{2.cm}
		\centering\includegraphics[width=2.cm]{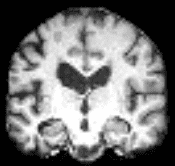}
	\end{subfigure}&
	\begin{subfigure}{2.cm}
		\centering\includegraphics[width=2.cm]{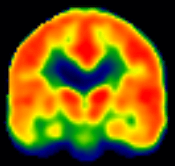}
	\end{subfigure}&
	\begin{subfigure}{2.cm}
		\centering\includegraphics[width=2.cm]{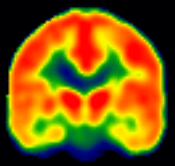}
	\end{subfigure}&
	
	\begin{subfigure}{2.cm}
		\centering\includegraphics[width=2.cm]{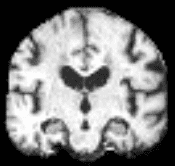}
	\end{subfigure}&
	\begin{subfigure}{2.cm}
		\centering\includegraphics[width=2.cm]{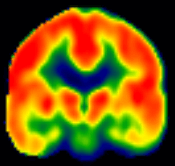}
	\end{subfigure}&
	\begin{subfigure}{2.cm}
		\centering\includegraphics[width=2.cm]{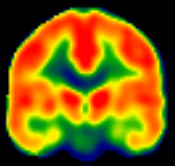}
	\end{subfigure} \\

	%%%%%%%%%%%%%%  c
			\begin{subfigure}{2.cm}
	\centering\includegraphics[width=2.cm]{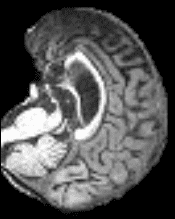}
\end{subfigure}&
\begin{subfigure}{2.cm}
	\centering\includegraphics[width=2.cm]{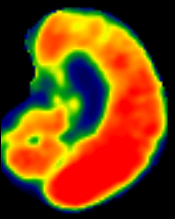}
\end{subfigure}&
\begin{subfigure}{2.cm}
	\centering\includegraphics[width=2.cm]{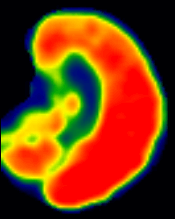}
\end{subfigure}&

\begin{subfigure}{2.cm}
	\centering\includegraphics[width=2.cm]{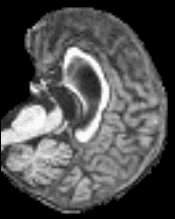}
\end{subfigure}&
\begin{subfigure}{2.cm}
	\centering\includegraphics[width=2.cm]{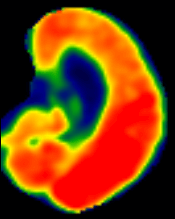}
\end{subfigure}&
\begin{subfigure}{2.cm}
	\centering\includegraphics[width=2.cm]{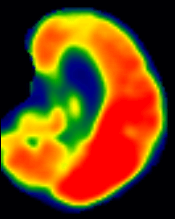}
\end{subfigure} \\

	\end{tabular}

	\caption{\label{fig:samples-ad} Two synthetic AD subjects. From left to right: input of MRI, the ground truth, the synthetic subject.}
\end{figure*}

%%%% CNs
\begin{figure*}[]
	\centering
	\begin{tabular}{ccc|ccc}
		MRI & GT & Synthetic & MRI & GT & Synthetic \\
		
		%%%%%%%%%%%%%%  s
		\begin{subfigure}{2.cm}
			\centering\includegraphics[width=2.cm]{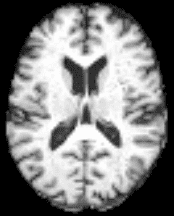}
		\end{subfigure}&
		\begin{subfigure}{2.cm}
			\centering\includegraphics[width=2.cm]{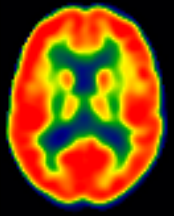}
		\end{subfigure}&
		\begin{subfigure}{2.cm}
			\centering\includegraphics[width=2.cm]{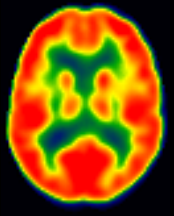}
		\end{subfigure}&
		
		\begin{subfigure}{2.cm}
			\centering\includegraphics[width=2.cm]{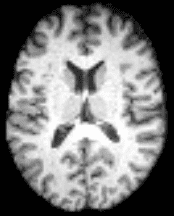}
		\end{subfigure}&
		\begin{subfigure}{2.cm}
			\centering\includegraphics[width=2.cm]{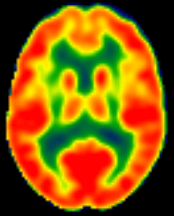}
		\end{subfigure}&
		\begin{subfigure}{2.cm}
			\centering\includegraphics[width=2.cm]{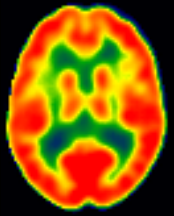}
		\end{subfigure} \\

		%%%%%%%%%%%%%%  a
		\begin{subfigure}{2.cm}
			\centering\includegraphics[width=2.cm]{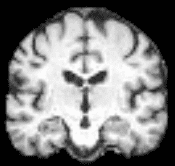}
		\end{subfigure}&
		\begin{subfigure}{2.cm}
			\centering\includegraphics[width=2.cm]{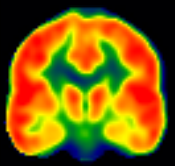}
		\end{subfigure}&
		\begin{subfigure}{2.cm}
			\centering\includegraphics[width=2.cm]{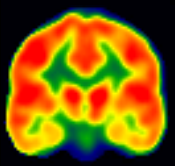}
		\end{subfigure}&
		
		\begin{subfigure}{2.cm}
			\centering\includegraphics[width=2.cm]{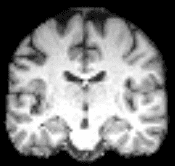}
		\end{subfigure}&
		\begin{subfigure}{2.cm}
			\centering\includegraphics[width=2.cm]{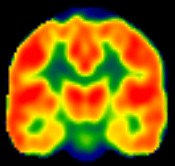}
		\end{subfigure}&
		\begin{subfigure}{2.cm}
			\centering\includegraphics[width=2.cm]{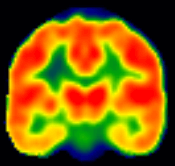}
		\end{subfigure} \\

		%%%%%%%%%%%%%%  c
		\begin{subfigure}{2.cm}
			\centering\includegraphics[width=2.cm]{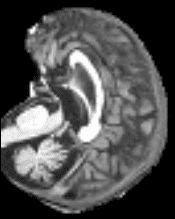}
		\end{subfigure}&
		\begin{subfigure}{2.cm}
			\centering\includegraphics[width=2.cm]{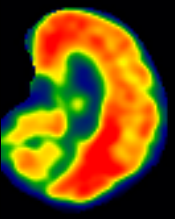}
		\end{subfigure}&
		\begin{subfigure}{2.cm}
			\centering\includegraphics[width=2.cm]{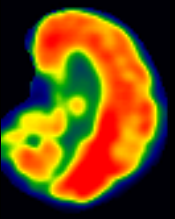}
		\end{subfigure}&
		
		\begin{subfigure}{2.cm}
			\centering\includegraphics[width=2.cm]{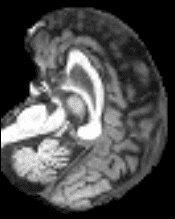}
		\end{subfigure}&
		\begin{subfigure}{2.cm}
			\centering\includegraphics[width=2.cm]{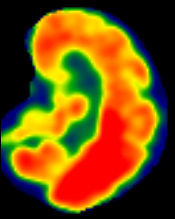}
		\end{subfigure}&
		\begin{subfigure}{2.cm}
			\centering\includegraphics[width=2.cm]{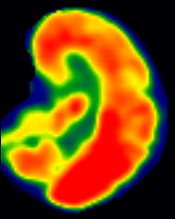}
		\end{subfigure} \\
		
	\end{tabular}

	\caption{\label{fig:samples-cn} Two synthetic CN subjects. From left to right: input of MRI, the ground truth, the synthetic subject.}
\end{figure*}

%%%% MCIs
\begin{figure*}[]
	\centering
	\begin{tabular}{ccc|ccc}
		MRI & GT & Synthetic & MRI & GT & Synthetic \\
		
		%%%%%%%%%%%%%%  s
		\begin{subfigure}{2.cm}
			\centering\includegraphics[width=2.cm]{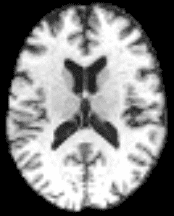}
		\end{subfigure}&
		\begin{subfigure}{2.cm}
			\centering\includegraphics[width=2.cm]{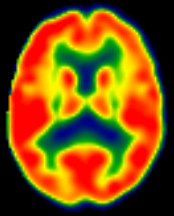}
		\end{subfigure}&
		\begin{subfigure}{2.cm}
			\centering\includegraphics[width=2.cm]{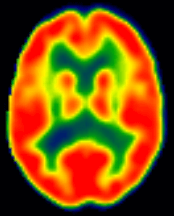}
		\end{subfigure}&
		
		\begin{subfigure}{2.cm}
			\centering\includegraphics[width=2.cm]{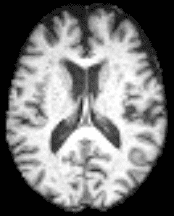}
		\end{subfigure}&
		\begin{subfigure}{2.cm}
			\centering\includegraphics[width=2.cm]{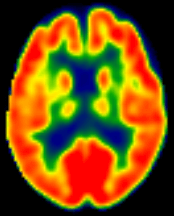}
		\end{subfigure}&
		\begin{subfigure}{2.cm}
			\centering\includegraphics[width=2.cm]{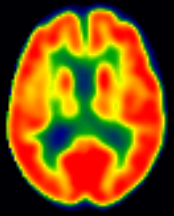}
		\end{subfigure} \\

		%%%%%%%%%%%%%%  a
		\begin{subfigure}{2.cm}
			\centering\includegraphics[width=2.cm]{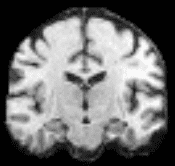}
		\end{subfigure}&
		\begin{subfigure}{2.cm}
			\centering\includegraphics[width=2.cm]{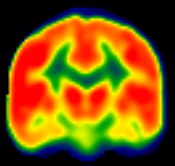}
		\end{subfigure}&
		\begin{subfigure}{2.cm}
			\centering\includegraphics[width=2.cm]{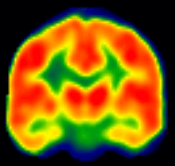}
		\end{subfigure}&
		
		\begin{subfigure}{2.cm}
			\centering\includegraphics[width=2.cm]{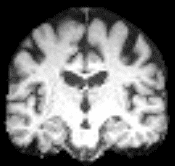}
		\end{subfigure}&
		\begin{subfigure}{2.cm}
			\centering\includegraphics[width=2.cm]{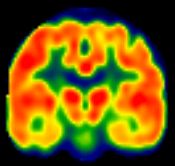}
		\end{subfigure}&
		\begin{subfigure}{2.cm}
			\centering\includegraphics[width=2.cm]{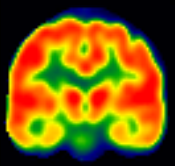}
		\end{subfigure} \\

		%%%%%%%%%%%%%%  c
		\begin{subfigure}{2.cm}
			\centering\includegraphics[width=2.cm]{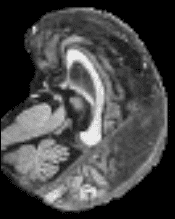}
		\end{subfigure}&
		\begin{subfigure}{2.cm}
			\centering\includegraphics[width=2.cm]{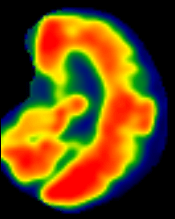}
		\end{subfigure}&
		\begin{subfigure}{2.cm}
			\centering\includegraphics[width=2.cm]{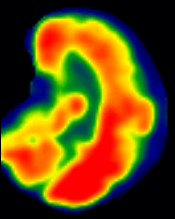}
		\end{subfigure}&
		
		\begin{subfigure}{2.cm}
			\centering\includegraphics[width=2.cm]{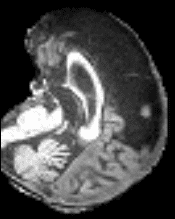}
		\end{subfigure}&
		\begin{subfigure}{2.cm}
			\centering\includegraphics[width=2.cm]{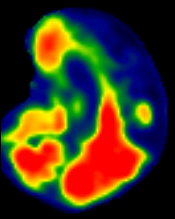}
		\end{subfigure}&
		\begin{subfigure}{2.cm}
			\centering\includegraphics[width=2.cm]{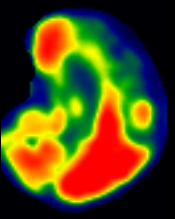}
		\end{subfigure} \\
		
	\end{tabular}

	\caption{\label{fig:samples-mci} Two synthetic MCI subjects. From left to right: input of MRI, the ground truth, the synthetic subject.}
\end{figure*}

%%%%%%%%%%%%%%%%%%%%%%%%%%%%%%%%% t-test %%%%%%%%%%%%%%%%%%%%%%%%%%%%%%
\begin{figure*}[]
	\centering
	\begin{subfigure}{3.1cm}
		\includegraphics[height=3.cm]{./figs/ttest-a.png}
	\end{subfigure}
	\begin{subfigure}{4.15 cm}
		\includegraphics[height=3.cm]{./figs/ttest-s.png}
	\end{subfigure}
	\begin{subfigure}{4.1 cm}
		\includegraphics[height=3.cm]{./figs/ttest-c.png}
	\end{subfigure}
	\caption{\label{fig:t-test} T-test for generated images(Purple red) and the ground truth (Yellow) in testing data. The large overlapping region illustrates the consistence in AD $\mid$ CN hypothesis testing.}
\end{figure*}

\begin{figure*}[t]
	\centering
	%\vspace{-8mm}
	\begin{tabular}{C{3mm} ccccccc}
		& MRI & 50 & 60 & 70 & 80 & 90 & 100 \\
		%%%%%%%%%%%%%%%%%%%%% ADs%%%%%%%%%%%%%%%%%%%%%%%%%%%%%%%
		%%%%%%%%%%%%%%  s&
		&
		\begin{subfigure}{1.5cm}
			\centering\includegraphics[width=1.5cm]{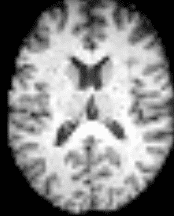}
		\end{subfigure} &
		\begin{subfigure}{1.5cm}
			\centering\includegraphics[width=1.5cm]{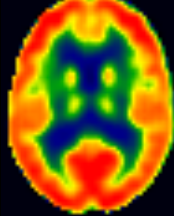}
		\end{subfigure}&
		\begin{subfigure}{1.5cm}
			\centering\includegraphics[width=1.5cm]{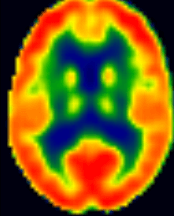}
		\end{subfigure}&
		\begin{subfigure}{1.5cm}
			\centering\includegraphics[width=1.5cm]{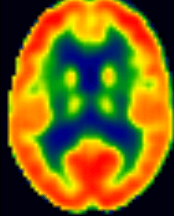}
		\end{subfigure}&
		
		\begin{subfigure}{1.5cm}
			\centering\includegraphics[width=1.5cm]{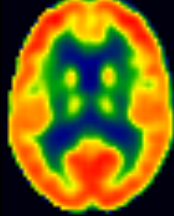}
		\end{subfigure}&
		\begin{subfigure}{1.5cm}
			\centering\includegraphics[width=1.5cm]{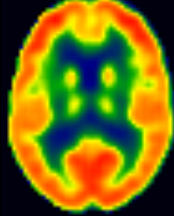}
		\end{subfigure}&
		\begin{subfigure}{1.5cm}
			\centering\includegraphics[width=1.5cm]{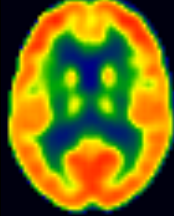}
		\end{subfigure}\\

		%%%%%%%%%%%%%%  a
		\multirow{3}{*}{AD}&
		\begin{subfigure}{1.5cm}
			\centering\includegraphics[width=1.5cm]{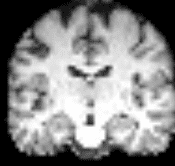}
		\end{subfigure} &
		\begin{subfigure}{1.5cm}
			\centering\includegraphics[width=1.5cm]{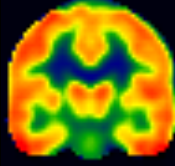}
		\end{subfigure}&
		\begin{subfigure}{1.5cm}
			\centering\includegraphics[width=1.5cm]{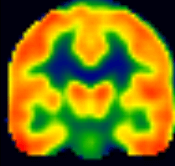}
		\end{subfigure}&
		\begin{subfigure}{1.5cm}
			\centering\includegraphics[width=1.5cm]{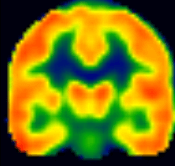}
		\end{subfigure}&
		
		\begin{subfigure}{1.5cm}
			\centering\includegraphics[width=1.5cm]{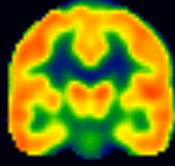}
		\end{subfigure}&
		\begin{subfigure}{1.5cm}
			\centering\includegraphics[width=1.5cm]{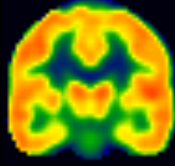}
		\end{subfigure}&
		\begin{subfigure}{1.5cm}
			\centering\includegraphics[width=1.5cm]{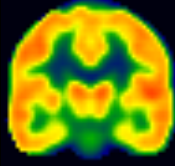}
		\end{subfigure}\\

		%%%%%%%%%%%%%%  c
		&
		\begin{subfigure}{1.5cm}
			\centering\includegraphics[width=1.5cm]{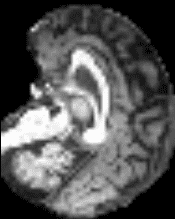}
		\end{subfigure} &
		\begin{subfigure}{1.5cm}
			\centering\includegraphics[width=1.5cm]{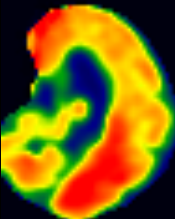}
		\end{subfigure}&
		\begin{subfigure}{1.5cm}
			\centering\includegraphics[width=1.5cm]{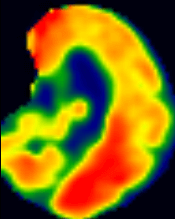}
		\end{subfigure}&
		\begin{subfigure}{1.5cm}
			\centering\includegraphics[width=1.5cm]{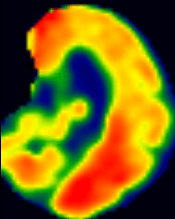}
		\end{subfigure}&
		
		\begin{subfigure}{1.5cm}
			\centering\includegraphics[width=1.5cm]{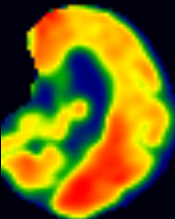}
		\end{subfigure}&
		\begin{subfigure}{1.5cm}
			\centering\includegraphics[width=1.5cm]{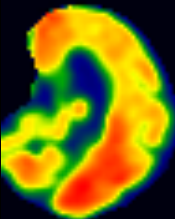}
		\end{subfigure}&
		\begin{subfigure}{1.5cm}
			\centering\includegraphics[width=1.5cm]{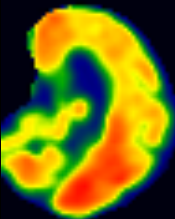}
		\end{subfigure}\\
		
		\vspace{-3mm}
		\\
		
		\hline
		\vspace{-3mm}
		\\
		
		%%%%%%%%%%%%%%%%%%%%% MCI %%%%%%%%%%%%%%%%%%%%%%%%%%%%%%%
		%%%%%%%%%%%%%%  s
		&
		\begin{subfigure}{1.5cm}
			\centering\includegraphics[width=1.5cm]{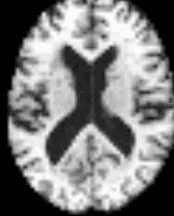}
		\end{subfigure}&
		\begin{subfigure}{1.5cm}
			\centering\includegraphics[width=1.5cm]{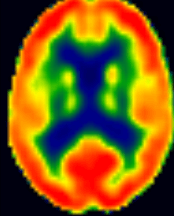}
		\end{subfigure}&
		\begin{subfigure}{1.5cm}
			\centering\includegraphics[width=1.5cm]{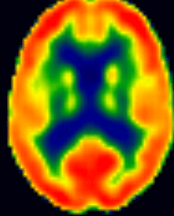}
		\end{subfigure}&
		\begin{subfigure}{1.5cm}
			\centering\includegraphics[width=1.5cm]{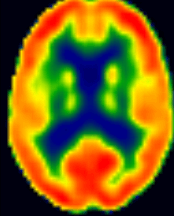}
		\end{subfigure}&
		
		\begin{subfigure}{1.5cm}
			\centering\includegraphics[width=1.5cm]{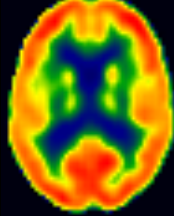}
		\end{subfigure}&
		\begin{subfigure}{1.5cm}
			\centering\includegraphics[width=1.5cm]{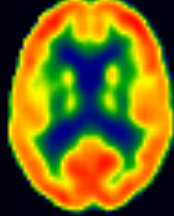}
		\end{subfigure}&
		\begin{subfigure}{1.5cm}
			\centering\includegraphics[width=1.5cm]{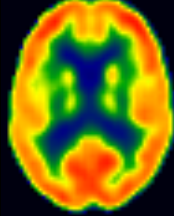}
		\end{subfigure} \\

		%%%%%%%%%%%%%%  a
		\multirow{3}{*}{MCI}&
		\begin{subfigure}{1.5cm}
			\centering\includegraphics[width=1.5cm]{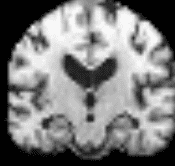}
		\end{subfigure} &
		\begin{subfigure}{1.5cm}
			\centering\includegraphics[width=1.5cm]{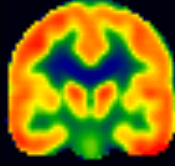}
		\end{subfigure}&
		\begin{subfigure}{1.5cm}
			\centering\includegraphics[width=1.5cm]{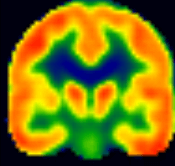}
		\end{subfigure}&
		\begin{subfigure}{1.5cm}
			\centering\includegraphics[width=1.5cm]{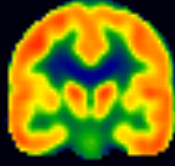}
		\end{subfigure}&
		
		\begin{subfigure}{1.5cm}
			\centering\includegraphics[width=1.5cm]{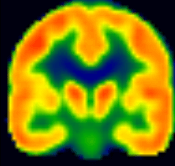}
		\end{subfigure}&
		\begin{subfigure}{1.5cm}
			\centering\includegraphics[width=1.5cm]{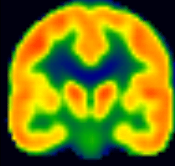}
		\end{subfigure}&
		\begin{subfigure}{1.5cm}
			\centering\includegraphics[width=1.5cm]{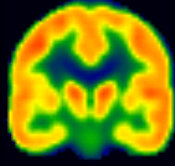}
		\end{subfigure}\\

		%%%%%%%%%%%%%%  c
		&
		\begin{subfigure}{1.5cm}
			\centering\includegraphics[width=1.5cm]{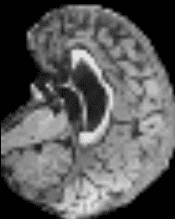}
		\end{subfigure} &
		\begin{subfigure}{1.5cm}
			\centering\includegraphics[width=1.5cm]{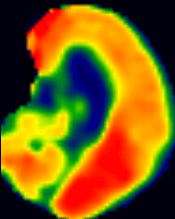}
		\end{subfigure}&
		\begin{subfigure}{1.5cm}
			\centering\includegraphics[width=1.5cm]{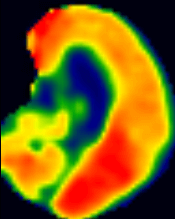}
		\end{subfigure}&
		\begin{subfigure}{1.5cm}
			\centering\includegraphics[width=1.5cm]{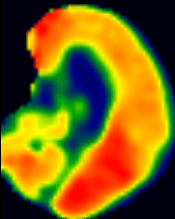}
		\end{subfigure}&
		
		\begin{subfigure}{1.5cm}
			\centering\includegraphics[width=1.5cm]{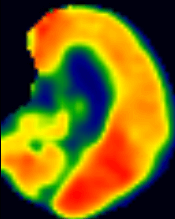}
		\end{subfigure}&
		\begin{subfigure}{1.5cm}
			\centering\includegraphics[width=1.5cm]{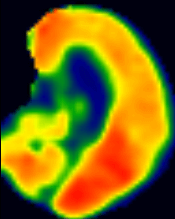}
		\end{subfigure}&
		\begin{subfigure}{1.5cm}
			\centering\includegraphics[width=1.5cm]{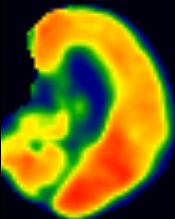}
		\end{subfigure}\\

		\vspace{-3mm}
		\\
		
		\hline
		\vspace{-3mm}
		\\
		%%%%%%%%%%%%%%%%%%%%% CN %%%%%%%%%%%%%%%%%%%%%%%%%%%%%%%
		%%%%%%%%%%%%%%  s
		&
		\begin{subfigure}{1.5cm}
			\centering\includegraphics[width=1.5cm]{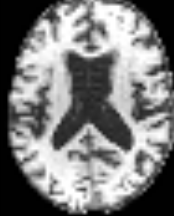}
		\end{subfigure} &
		\begin{subfigure}{1.5cm}
			\centering\includegraphics[width=1.5cm]{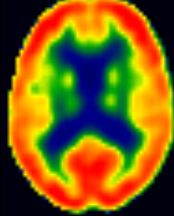}
		\end{subfigure}&
		\begin{subfigure}{1.5cm}
			\centering\includegraphics[width=1.5cm]{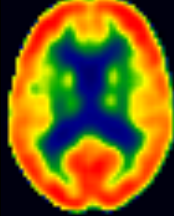}
		\end{subfigure}&
		\begin{subfigure}{1.5cm}
			\centering\includegraphics[width=1.5cm]{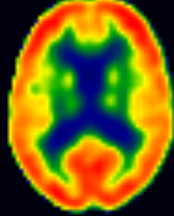}
		\end{subfigure}&
		
		\begin{subfigure}{1.5cm}
			\centering\includegraphics[width=1.5cm]{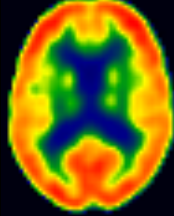}
		\end{subfigure}&
		\begin{subfigure}{1.5cm}
			\centering\includegraphics[width=1.5cm]{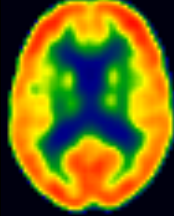}
		\end{subfigure}&
		\begin{subfigure}{1.5cm}
			\centering\includegraphics[width=1.5cm]{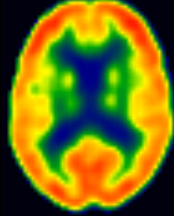}
		\end{subfigure}\\

		%%%%%%%%%%%%%%  a
		\multirow{3}{*}{CN}&
		\begin{subfigure}{1.5cm}
			\centering\includegraphics[width=1.5cm]{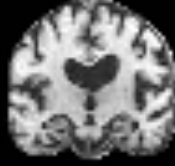}
		\end{subfigure} &
		\begin{subfigure}{1.5cm}
			\centering\includegraphics[width=1.5cm]{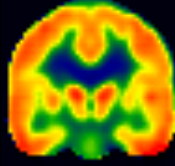}
		\end{subfigure}&
		\begin{subfigure}{1.5cm}
			\centering\includegraphics[width=1.5cm]{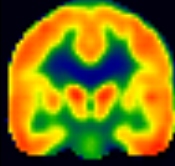}
		\end{subfigure}&
		\begin{subfigure}{1.5cm}
			\centering\includegraphics[width=1.5cm]{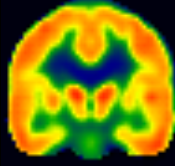}
		\end{subfigure}&
		
		\begin{subfigure}{1.5cm}
			\centering\includegraphics[width=1.5cm]{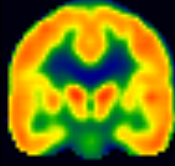}
		\end{subfigure}&
		\begin{subfigure}{1.5cm}
			\centering\includegraphics[width=1.5cm]{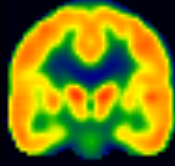}
		\end{subfigure}&
		\begin{subfigure}{1.5cm}
			\centering\includegraphics[width=1.5cm]{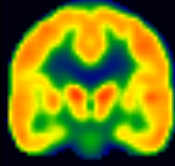}
		\end{subfigure}\\

		%%%%%%%%%%%%%%  c
		&
		\begin{subfigure}{1.5cm}
			\centering\includegraphics[width=1.5cm]{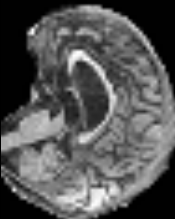}
		\end{subfigure} &
		\begin{subfigure}{1.5cm}
			\centering\includegraphics[width=1.5cm]{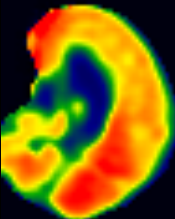}
		\end{subfigure}&
		\begin{subfigure}{1.5cm}
			\centering\includegraphics[width=1.5cm]{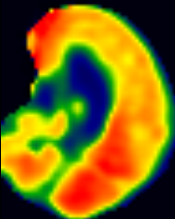}
		\end{subfigure}&
		\begin{subfigure}{1.5cm}
			\centering\includegraphics[width=1.5cm]{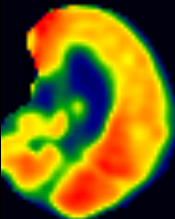}
		\end{subfigure}&
		
		\begin{subfigure}{1.5cm}
			\centering\includegraphics[width=1.5cm]{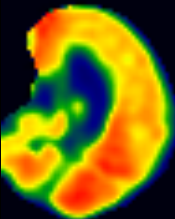}
		\end{subfigure}&
		\begin{subfigure}{1.5cm}
			\centering\includegraphics[width=1.5cm]{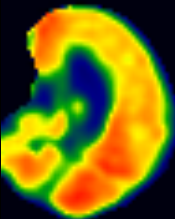}
		\end{subfigure}&
		\begin{subfigure}{1.5cm}
			\centering\includegraphics[width=1.5cm]{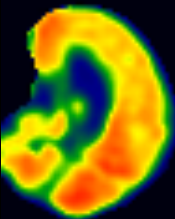}
		\end{subfigure}\\
		
	\end{tabular}

	\caption{\label{fig:cond_samples} Age information manipulation. There are 3 subjects, AD, MCI, and CN, each subject provides $6$ results \textit{w.r.t.} a variant of age labels.}
\end{figure*}

\begin{figure*}[h]
	\centering
	\includegraphics[width=.8\textwidth]{./figs/cond_quan.eps}
	\vspace{-4mm}
	\caption{\label{fig:cond_quan} The mean intensity of $12$ ROIs with the change of age for $3$ average subjects.}
\end{figure*}
