# Supplementary material for: DUAL-GLOW: Conditional Flow-Based Generative Model for Modality Transfer
Source: arXiv:1908.08074 source file (2019-08-21)
Supplement: Supplementary file 2 [file exps-supp.tex]

\section{Experiments}

As a simple test, we first demonstrate DUAL-GLOWs ability to generate images on a standard computer vision modality transfer task. Using the UT-Zap50K dataset \cite{?} of shoe images, we construct HED \cite{?} edge images as ``sketches", similar to \cite{?}. We aim to learn a mapping from sketch to shoe. Figure \ref{fig:shoe} shows the results of applying our framework next to the ground truth. 
\begin{figure}
	\centering
	\text{\qquad\quad Sketch}\hfill\text{\quad Generated}\hfill\text{Ground Truth \quad}
	\vspace{5pt}
	
	\includegraphics[width=0.25\columnwidth]{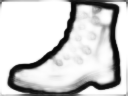}
	\hspace{5pt}\vrule\hspace{5pt}%
	\includegraphics[width=0.25\columnwidth]{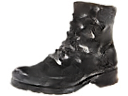}
	\hspace{5pt}\vrule\hspace{5pt}%
	\includegraphics[width=0.25\columnwidth]{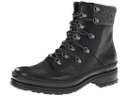}
	\caption{A sample generation using our DUAL-GLOWs framework learned on the UT-Zap50K dataset \cite{?}.}
\end{figure}

We evaluate the model's efficacy on the ADNI dataset both against ground truth images and in downstream application. We conduct extensive quantitative experiments to show that DUAL-GLOWs outperforms the baseline method consistently. Downstream, generated PET images show desirable properties in Alzheimer's Disease diagnosis. The conditional framework also shows extensibility in the prediction and tracking of age.

\subsection{Alzheimer's Disease Neuroimaging Initiative Dataset}
The Alzheimer's Disease Neuroimaging Initiative (ADNI)
provides a large database of studies
directly aimed at understanding the 
development and pathology of AD. Subjects are diagnosed as cognitively normal (CN), significant memory concern (SMC), early mild cognitive impairment (EMCI), mild cognitive impairment (MCI), late mild cognitive impairment (LMCI) or having Alzheimer's Disease (AD).
FDG-PET and T1-weighted MR images were
obtained from ADNI,
and pairs were constructed
by matching images
with the same subject ID 
and similar acquisition dates.

Images were processed using SPM12 \cite{ashburner2014spm12}. First, PET images were aligned to the paired MRI using coregistration. Next, MR images were nonlinearly mapped
to the MNI152 template.
Finally, PET images were mapped to the standard MNI space using the same forward warping identified in the MR segmentation step.
Voxel size was fixed for all volumes to 
$1.5\times 1.5 \times 1.5 \:  mm^3$,
and the final volume size obtained for 
both MR and PET images was $64 \times 96 \times 64$.
Through this procedure we finally
obtain 806 MRI/PET clean pairs. The demographics of the dataset are shown in Table \ref{demographics}. In our following experiments, we randomly select 726 objects as the training data and the remaining 80 as testing.

\begin{table*}[t]
	\begin{center}
		\caption{\label{demographics} Demographic details of the ADNI dataset.}
		\begin{tabular}{l  c    c c ccc}
			\hline
			\footnotesize{CATEGORY}     & CN    &SMC  &EMCI &MCI&LMCI &AD \\
			\hline                                                  
			\# of subjects          &$ 259$ &   $18$ & $88$ &  $263$ & $64$ & $114$ \\
			Age (mean)                &$76.47$ & $70.94$ & $71.64$ & $77.86$ & $73.14$ & $75.98$ \\
			Age (std)                &$5.26$ & $4.76$ & $6.55$ & $7.42$ & $6.43$ & $7.27$ \\
			Gender (F/M)             &$116/143$ & $11/7$ & $38/50$ & $66/197$ & $24/40$ & $42/72$ \\
					
			\hline
		\end{tabular}
	\end{center}
\end{table*}

\subsection{Framework Details}
The DUAL-GLOWs architecture outlined above was trained using Nvidia P100 GPUs with Tensorflow. There are $4$ ``levels" in our invertible network, each containing $16$ affine coupling layers. The nonlinear operators $\textrm{s}(\cdot)$ and $\textrm{t}(\cdot)$ are small networks with three 3D convolutional layers. For the hierarchical correction learning network, we split the hidden codes of the output of the first three modules in the invertible network and design four 3D convolutional networks for all latent codes. For the conditional framework case, we concatenate the five discriminators on the tail of all four levels of the MRI inference network and the top-most level of the PET inference network. The GRL is added between the inference network and the first three discriminators. The hyperparameter $lambda$ of the regularizer is set to $0.001$. For all classification losses, we give the weight of $0.01$. 

The model was trained using the AdamMax optimizer with an initial learning rate set to $0.001$ and exponential decay rates $0.9$ for the moment estimates. We train the model for $90$ epochs.

%%% suvr
%\begin{figure}[]
%	\centering
%	\includegraphics[width=0.98\columnwidth]{./figs/suvr.eps}
%	\caption{\label{fig:suvr} The relative SUVRs for 16 ROIs. }
%\end{figure}

%%% mae
%\begin{figure}[]
%	\includegraphics[width=0.98\columnwidth]{./figs/corr.pdf}
%	\caption{\label{fig:exp2} Mean absolute error on held out test set generations, stratified by age, sex, and disease status.}
%\end{figure}

%%%%%%%%%%%%%%%%%%%%%%%%%%%%%%%%%%%%%%% demogra %%%%%%%%%%%%%%%%%%%%%%%%%%%
%\begin{figure}[]
%	\centering
%	\begin{subfigure}{7.5cm}
%		\centering\includegraphics[width=7.5cm]{./figs/demogra-1.png}
%	\end{subfigure}
%	\begin{subfigure}{5.5cm}
%		\centering\includegraphics[width=5.5cm]{./figs/demogra-2.png}
%	\end{subfigure}
%	\caption{\label{fig:demographics} Demographics of all individuals included in our experiments. All information was collected from metadata provided by ADNI.}
%\end{figure}

%%%%%%%%%%%%%%%%%%%%%%%%%%%%%%%%% samples %%%%%%%%%%%%%%%%%%%%%%%%%%%%%%
%%%% ADs
\begin{figure*}[]
	\centering
	\begin{tabular}{ccc|ccc}
		MRI & GroundTruth & Synthetic & MRI & GroundTruth & Synthetic \\
		
		%%%%%%%%%%%%%%  s
		\begin{subfigure}{2.cm}
			\centering\includegraphics[width=2.cm]{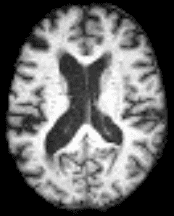}
		\end{subfigure}&
	\begin{subfigure}{2.cm}
		\centering\includegraphics[width=2.cm]{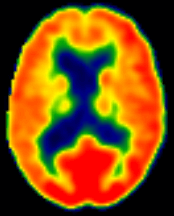}
	\end{subfigure}&
\begin{subfigure}{2.cm}
	\centering\includegraphics[width=2.cm]{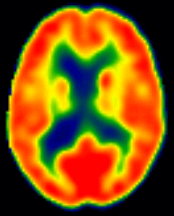}
\end{subfigure}&

	\begin{subfigure}{2.cm}
	\centering\includegraphics[width=2.cm]{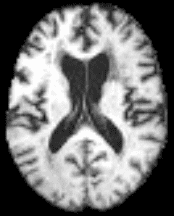}
\end{subfigure}&
\begin{subfigure}{2.cm}
	\centering\includegraphics[width=2.cm]{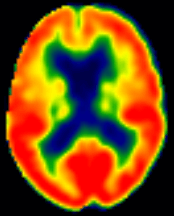}
\end{subfigure}&
\begin{subfigure}{2.cm}
	\centering\includegraphics[width=2.cm]{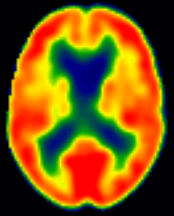}
\end{subfigure} \\

		%%%%%%%%%%%%%%  a
			\begin{subfigure}{2.cm}
		\centering\includegraphics[width=2.cm]{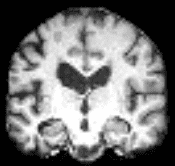}
	\end{subfigure}&
	\begin{subfigure}{2.cm}
		\centering\includegraphics[width=2.cm]{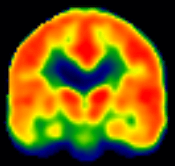}
	\end{subfigure}&
	\begin{subfigure}{2.cm}
		\centering\includegraphics[width=2.cm]{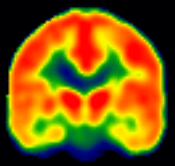}
	\end{subfigure}&
	
	\begin{subfigure}{2.cm}
		\centering\includegraphics[width=2.cm]{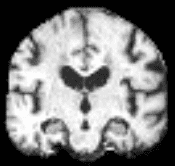}
	\end{subfigure}&
	\begin{subfigure}{2.cm}
		\centering\includegraphics[width=2.cm]{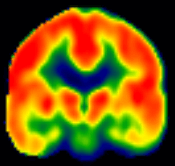}
	\end{subfigure}&
	\begin{subfigure}{2.cm}
		\centering\includegraphics[width=2.cm]{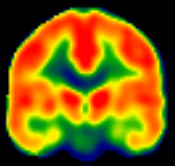}
	\end{subfigure} \\

	%%%%%%%%%%%%%%  c
			\begin{subfigure}{2.cm}
	\centering\includegraphics[width=2.cm]{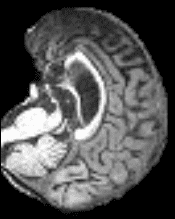}
\end{subfigure}&
\begin{subfigure}{2.cm}
	\centering\includegraphics[width=2.cm]{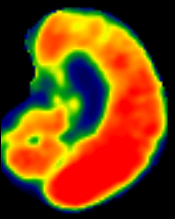}
\end{subfigure}&
\begin{subfigure}{2.cm}
	\centering\includegraphics[width=2.cm]{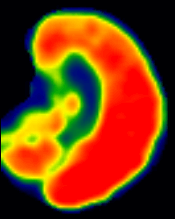}
\end{subfigure}&

\begin{subfigure}{2.cm}
	\centering\includegraphics[width=2.cm]{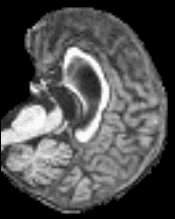}
\end{subfigure}&
\begin{subfigure}{2.cm}
	\centering\includegraphics[width=2.cm]{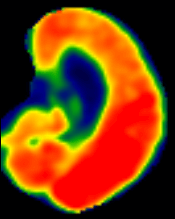}
\end{subfigure}&
\begin{subfigure}{2.cm}
	\centering\includegraphics[width=2.cm]{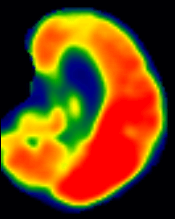}
\end{subfigure} \\

	\end{tabular}

	\caption{\label{fig:samples-ad} Synthetic images are meaningful for subjects in both
		extremes of disease spectrum. Two synthetic AD subjects. From left to right: input of MRI, the ground truth, the synthetic subject.}
\end{figure*}

%%%% CNs
\begin{figure*}[]
	\centering
	\begin{tabular}{ccc|ccc}
		MRI & GT & Synthetic & MRI & GT & Synthetic \\
		
		%%%%%%%%%%%%%%  s
		\begin{subfigure}{2.cm}
			\centering\includegraphics[width=2.cm]{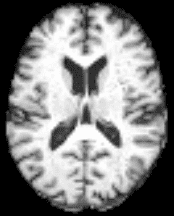}
		\end{subfigure}&
		\begin{subfigure}{2.cm}
			\centering\includegraphics[width=2.cm]{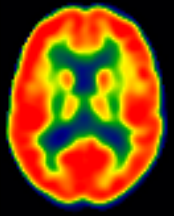}
		\end{subfigure}&
		\begin{subfigure}{2.cm}
			\centering\includegraphics[width=2.cm]{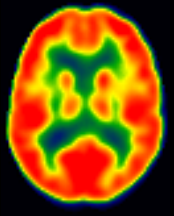}
		\end{subfigure}&
		
		\begin{subfigure}{2.cm}
			\centering\includegraphics[width=2.cm]{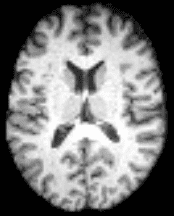}
		\end{subfigure}&
		\begin{subfigure}{2.cm}
			\centering\includegraphics[width=2.cm]{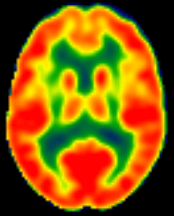}
		\end{subfigure}&
		\begin{subfigure}{2.cm}
			\centering\includegraphics[width=2.cm]{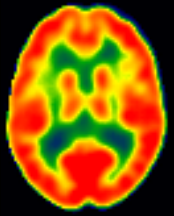}
		\end{subfigure} \\

		%%%%%%%%%%%%%%  a
		\begin{subfigure}{2.cm}
			\centering\includegraphics[width=2.cm]{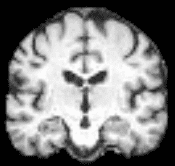}
		\end{subfigure}&
		\begin{subfigure}{2.cm}
			\centering\includegraphics[width=2.cm]{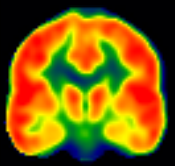}
		\end{subfigure}&
		\begin{subfigure}{2.cm}
			\centering\includegraphics[width=2.cm]{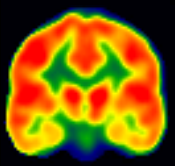}
		\end{subfigure}&
		
		\begin{subfigure}{2.cm}
			\centering\includegraphics[width=2.cm]{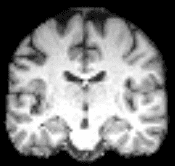}
		\end{subfigure}&
		\begin{subfigure}{2.cm}
			\centering\includegraphics[width=2.cm]{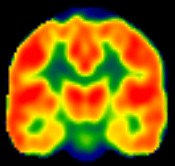}
		\end{subfigure}&
		\begin{subfigure}{2.cm}
			\centering\includegraphics[width=2.cm]{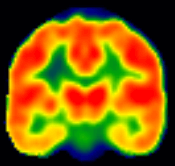}
		\end{subfigure} \\

		%%%%%%%%%%%%%%  c
		\begin{subfigure}{2.cm}
			\centering\includegraphics[width=2.cm]{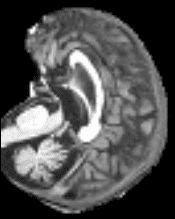}
		\end{subfigure}&
		\begin{subfigure}{2.cm}
			\centering\includegraphics[width=2.cm]{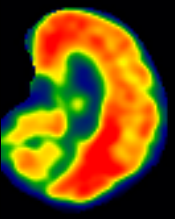}
		\end{subfigure}&
		\begin{subfigure}{2.cm}
			\centering\includegraphics[width=2.cm]{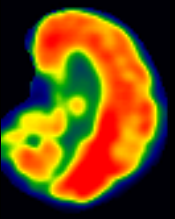}
		\end{subfigure}&
		
		\begin{subfigure}{2.cm}
			\centering\includegraphics[width=2.cm]{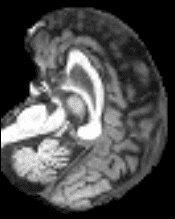}
		\end{subfigure}&
		\begin{subfigure}{2.cm}
			\centering\includegraphics[width=2.cm]{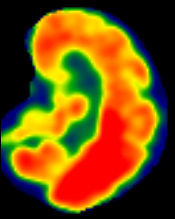}
		\end{subfigure}&
		\begin{subfigure}{2.cm}
			\centering\includegraphics[width=2.cm]{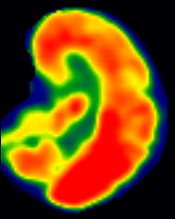}
		\end{subfigure} \\
		
	\end{tabular}

	\caption{\label{fig:samples-cn} Two synthetic CN subjects. From left to right: input of MRI, the ground truth, the synthetic subject.}
\end{figure*}

%%%% MCIs
\begin{figure*}[]
	\centering
	\begin{tabular}{ccc|ccc}
		MRI & GT & Synthetic & MRI & GT & Synthetic \\
		
		%%%%%%%%%%%%%%  s
		\begin{subfigure}{2.cm}
			\centering\includegraphics[width=2.cm]{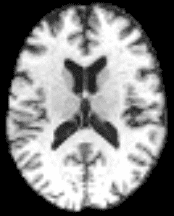}
		\end{subfigure}&
		\begin{subfigure}{2.cm}
			\centering\includegraphics[width=2.cm]{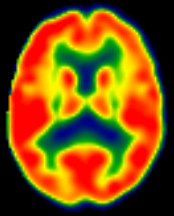}
		\end{subfigure}&
		\begin{subfigure}{2.cm}
			\centering\includegraphics[width=2.cm]{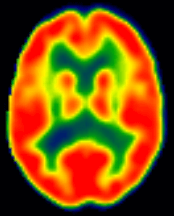}
		\end{subfigure}&
		
		\begin{subfigure}{2.cm}
			\centering\includegraphics[width=2.cm]{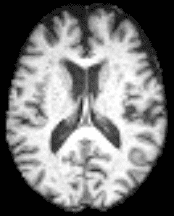}
		\end{subfigure}&
		\begin{subfigure}{2.cm}
			\centering\includegraphics[width=2.cm]{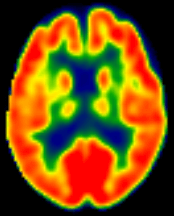}
		\end{subfigure}&
		\begin{subfigure}{2.cm}
			\centering\includegraphics[width=2.cm]{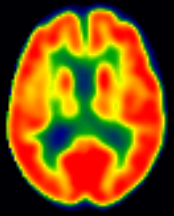}
		\end{subfigure} \\

		%%%%%%%%%%%%%%  a
		\begin{subfigure}{2.cm}
			\centering\includegraphics[width=2.cm]{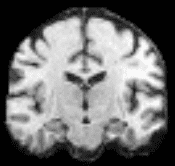}
		\end{subfigure}&
		\begin{subfigure}{2.cm}
			\centering\includegraphics[width=2.cm]{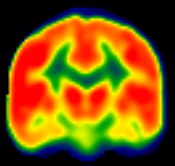}
		\end{subfigure}&
		\begin{subfigure}{2.cm}
			\centering\includegraphics[width=2.cm]{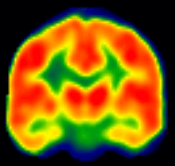}
		\end{subfigure}&
		
		\begin{subfigure}{2.cm}
			\centering\includegraphics[width=2.cm]{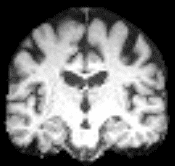}
		\end{subfigure}&
		\begin{subfigure}{2.cm}
			\centering\includegraphics[width=2.cm]{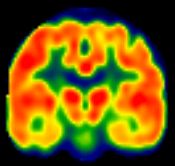}
		\end{subfigure}&
		\begin{subfigure}{2.cm}
			\centering\includegraphics[width=2.cm]{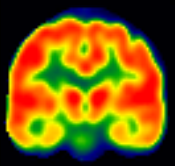}
		\end{subfigure} \\

		%%%%%%%%%%%%%%  c
		\begin{subfigure}{2.cm}
			\centering\includegraphics[width=2.cm]{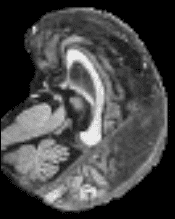}
		\end{subfigure}&
		\begin{subfigure}{2.cm}
			\centering\includegraphics[width=2.cm]{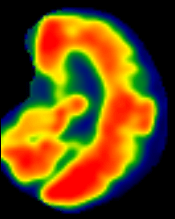}
		\end{subfigure}&
		\begin{subfigure}{2.cm}
			\centering\includegraphics[width=2.cm]{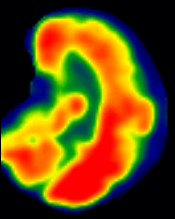}
		\end{subfigure}&
		
		\begin{subfigure}{2.cm}
			\centering\includegraphics[width=2.cm]{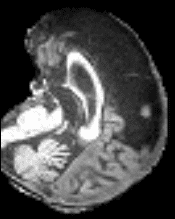}
		\end{subfigure}&
		\begin{subfigure}{2.cm}
			\centering\includegraphics[width=2.cm]{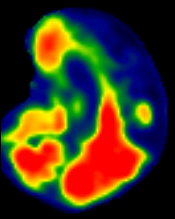}
		\end{subfigure}&
		\begin{subfigure}{2.cm}
			\centering\includegraphics[width=2.cm]{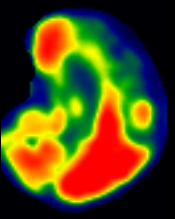}
		\end{subfigure} \\
		
	\end{tabular}

	\caption{\label{fig:samples-mci} Two synthetic MCI subjects. From left to right: input of MRI, the ground truth, the synthetic subject.}
\end{figure*}

%%%%%%%%%%%%%%%%%%%%%%%%%%%%%%%%% t-test %%%%%%%%%%%%%%%%%%%%%%%%%%%%%%
\begin{figure*}[]
	\centering
	\begin{subfigure}{3.1cm}
		\includegraphics[height=3.cm]{./figs/ttest-a.png}
	\end{subfigure}
	\begin{subfigure}{4.15 cm}
		\includegraphics[height=3.cm]{./figs/ttest-s.png}
	\end{subfigure}
	\begin{subfigure}{4.1 cm}
		\includegraphics[height=3.cm]{./figs/ttest-c.png}
	\end{subfigure}
	\caption{\label{fig:t-test} T-test for generated images(Purple red) and the ground truth (Yellow) in testing data. The large overlapping region illustrates the consistence in AD $\mid$ CN hypothesis testing.}
\end{figure*}

\begin{figure*}[t]
	\centering
	%\vspace{-8mm}
	\begin{tabular}{C{3mm} ccccccc}
		& MRI & 50 & 60 & 70 & 80 & 90 & 100 \\
		%%%%%%%%%%%%%%%%%%%%% ADs%%%%%%%%%%%%%%%%%%%%%%%%%%%%%%%
		%%%%%%%%%%%%%%  s&
		&
		\begin{subfigure}{1.5cm}
			\centering\includegraphics[width=1.5cm]{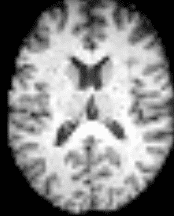}
		\end{subfigure} &
		\begin{subfigure}{1.5cm}
			\centering\includegraphics[width=1.5cm]{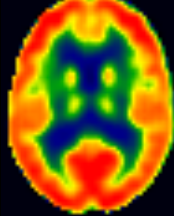}
		\end{subfigure}&
		\begin{subfigure}{1.5cm}
			\centering\includegraphics[width=1.5cm]{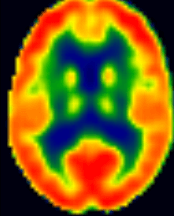}
		\end{subfigure}&
		\begin{subfigure}{1.5cm}
			\centering\includegraphics[width=1.5cm]{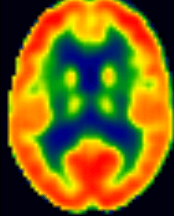}
		\end{subfigure}&
		
		\begin{subfigure}{1.5cm}
			\centering\includegraphics[width=1.5cm]{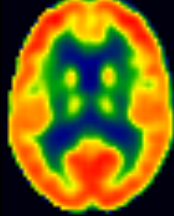}
		\end{subfigure}&
		\begin{subfigure}{1.5cm}
			\centering\includegraphics[width=1.5cm]{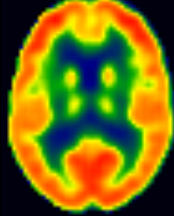}
		\end{subfigure}&
		\begin{subfigure}{1.5cm}
			\centering\includegraphics[width=1.5cm]{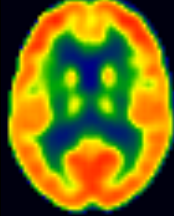}
		\end{subfigure}\\

		%%%%%%%%%%%%%%  a
		\multirow{3}{*}{AD}&
		\begin{subfigure}{1.5cm}
			\centering\includegraphics[width=1.5cm]{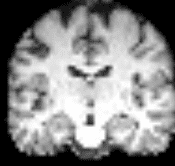}
		\end{subfigure} &
		\begin{subfigure}{1.5cm}
			\centering\includegraphics[width=1.5cm]{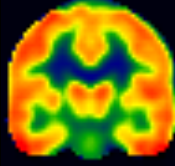}
		\end{subfigure}&
		\begin{subfigure}{1.5cm}
			\centering\includegraphics[width=1.5cm]{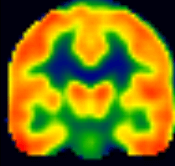}
		\end{subfigure}&
		\begin{subfigure}{1.5cm}
			\centering\includegraphics[width=1.5cm]{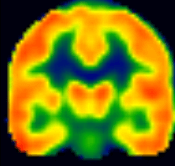}
		\end{subfigure}&
		
		\begin{subfigure}{1.5cm}
			\centering\includegraphics[width=1.5cm]{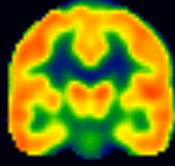}
		\end{subfigure}&
		\begin{subfigure}{1.5cm}
			\centering\includegraphics[width=1.5cm]{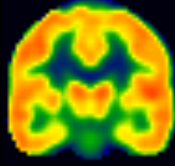}
		\end{subfigure}&
		\begin{subfigure}{1.5cm}
			\centering\includegraphics[width=1.5cm]{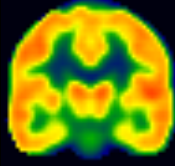}
		\end{subfigure}\\

		%%%%%%%%%%%%%%  c
		&
		\begin{subfigure}{1.5cm}
			\centering\includegraphics[width=1.5cm]{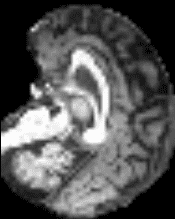}
		\end{subfigure} &
		\begin{subfigure}{1.5cm}
			\centering\includegraphics[width=1.5cm]{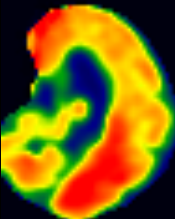}
		\end{subfigure}&
		\begin{subfigure}{1.5cm}
			\centering\includegraphics[width=1.5cm]{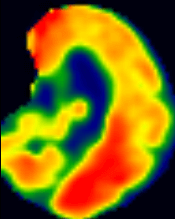}
		\end{subfigure}&
		\begin{subfigure}{1.5cm}
			\centering\includegraphics[width=1.5cm]{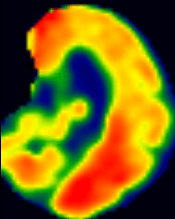}
		\end{subfigure}&
		
		\begin{subfigure}{1.5cm}
			\centering\includegraphics[width=1.5cm]{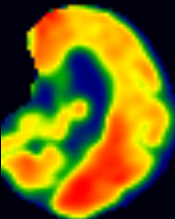}
		\end{subfigure}&
		\begin{subfigure}{1.5cm}
			\centering\includegraphics[width=1.5cm]{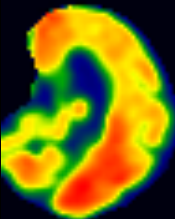}
		\end{subfigure}&
		\begin{subfigure}{1.5cm}
			\centering\includegraphics[width=1.5cm]{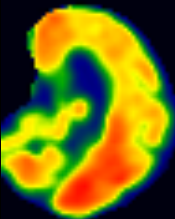}
		\end{subfigure}\\
		
		\vspace{-3mm}
		\\
		
		\hline
		\vspace{-3mm}
		\\
		
		%%%%%%%%%%%%%%%%%%%%% MCI %%%%%%%%%%%%%%%%%%%%%%%%%%%%%%%
		%%%%%%%%%%%%%%  s
		&
		\begin{subfigure}{1.5cm}
			\centering\includegraphics[width=1.5cm]{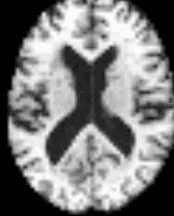}
		\end{subfigure}&
		\begin{subfigure}{1.5cm}
			\centering\includegraphics[width=1.5cm]{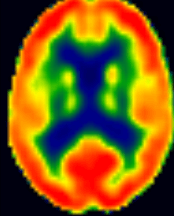}
		\end{subfigure}&
		\begin{subfigure}{1.5cm}
			\centering\includegraphics[width=1.5cm]{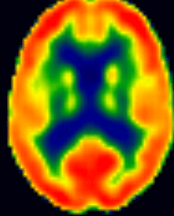}
		\end{subfigure}&
		\begin{subfigure}{1.5cm}
			\centering\includegraphics[width=1.5cm]{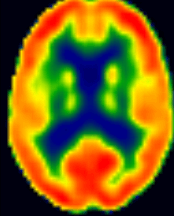}
		\end{subfigure}&
		
		\begin{subfigure}{1.5cm}
			\centering\includegraphics[width=1.5cm]{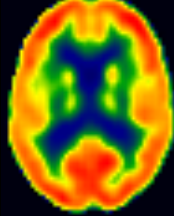}
		\end{subfigure}&
		\begin{subfigure}{1.5cm}
			\centering\includegraphics[width=1.5cm]{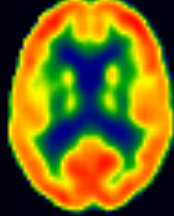}
		\end{subfigure}&
		\begin{subfigure}{1.5cm}
			\centering\includegraphics[width=1.5cm]{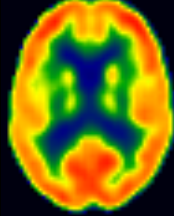}
		\end{subfigure} \\

		%%%%%%%%%%%%%%  a
		\multirow{3}{*}{MCI}&
		\begin{subfigure}{1.5cm}
			\centering\includegraphics[width=1.5cm]{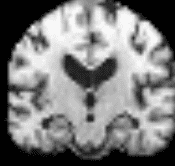}
		\end{subfigure} &
		\begin{subfigure}{1.5cm}
			\centering\includegraphics[width=1.5cm]{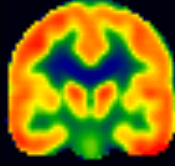}
		\end{subfigure}&
		\begin{subfigure}{1.5cm}
			\centering\includegraphics[width=1.5cm]{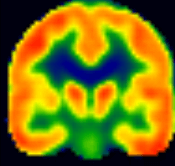}
		\end{subfigure}&
		\begin{subfigure}{1.5cm}
			\centering\includegraphics[width=1.5cm]{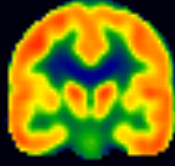}
		\end{subfigure}&
		
		\begin{subfigure}{1.5cm}
			\centering\includegraphics[width=1.5cm]{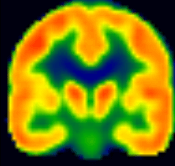}
		\end{subfigure}&
		\begin{subfigure}{1.5cm}
			\centering\includegraphics[width=1.5cm]{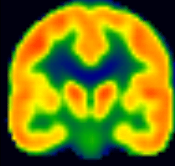}
		\end{subfigure}&
		\begin{subfigure}{1.5cm}
			\centering\includegraphics[width=1.5cm]{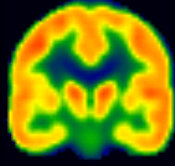}
		\end{subfigure}\\

		%%%%%%%%%%%%%%  c
		&
		\begin{subfigure}{1.5cm}
			\centering\includegraphics[width=1.5cm]{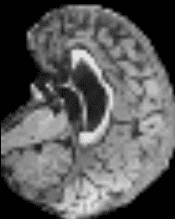}
		\end{subfigure} &
		\begin{subfigure}{1.5cm}
			\centering\includegraphics[width=1.5cm]{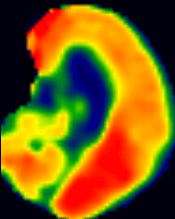}
		\end{subfigure}&
		\begin{subfigure}{1.5cm}
			\centering\includegraphics[width=1.5cm]{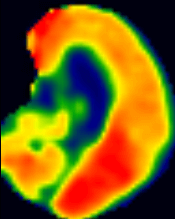}
		\end{subfigure}&
		\begin{subfigure}{1.5cm}
			\centering\includegraphics[width=1.5cm]{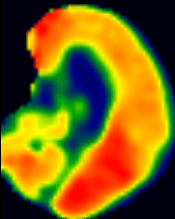}
		\end{subfigure}&
		
		\begin{subfigure}{1.5cm}
			\centering\includegraphics[width=1.5cm]{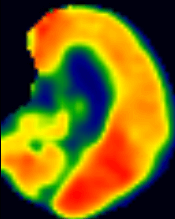}
		\end{subfigure}&
		\begin{subfigure}{1.5cm}
			\centering\includegraphics[width=1.5cm]{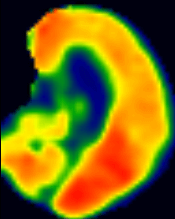}
		\end{subfigure}&
		\begin{subfigure}{1.5cm}
			\centering\includegraphics[width=1.5cm]{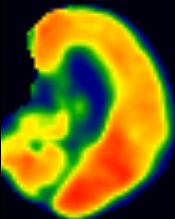}
		\end{subfigure}\\

		\vspace{-3mm}
		\\
		
		\hline
		\vspace{-3mm}
		\\
		%%%%%%%%%%%%%%%%%%%%% CN %%%%%%%%%%%%%%%%%%%%%%%%%%%%%%%
		%%%%%%%%%%%%%%  s
		&
		\begin{subfigure}{1.5cm}
			\centering\includegraphics[width=1.5cm]{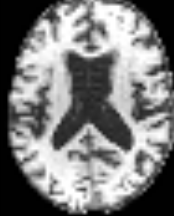}
		\end{subfigure} &
		\begin{subfigure}{1.5cm}
			\centering\includegraphics[width=1.5cm]{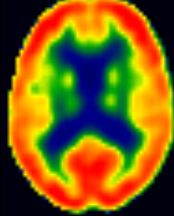}
		\end{subfigure}&
		\begin{subfigure}{1.5cm}
			\centering\includegraphics[width=1.5cm]{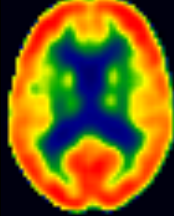}
		\end{subfigure}&
		\begin{subfigure}{1.5cm}
			\centering\includegraphics[width=1.5cm]{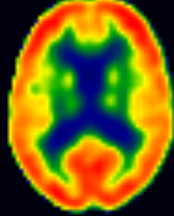}
		\end{subfigure}&
		
		\begin{subfigure}{1.5cm}
			\centering\includegraphics[width=1.5cm]{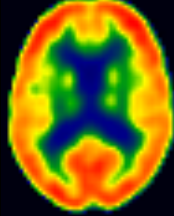}
		\end{subfigure}&
		\begin{subfigure}{1.5cm}
			\centering\includegraphics[width=1.5cm]{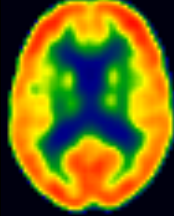}
		\end{subfigure}&
		\begin{subfigure}{1.5cm}
			\centering\includegraphics[width=1.5cm]{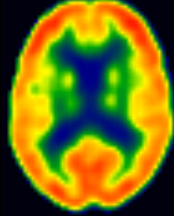}
		\end{subfigure}\\

		%%%%%%%%%%%%%%  a
		\multirow{3}{*}{CN}&
		\begin{subfigure}{1.5cm}
			\centering\includegraphics[width=1.5cm]{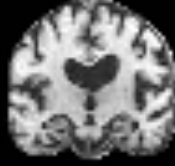}
		\end{subfigure} &
		\begin{subfigure}{1.5cm}
			\centering\includegraphics[width=1.5cm]{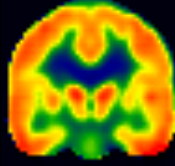}
		\end{subfigure}&
		\begin{subfigure}{1.5cm}
			\centering\includegraphics[width=1.5cm]{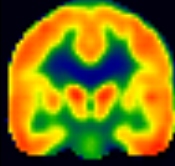}
		\end{subfigure}&
		\begin{subfigure}{1.5cm}
			\centering\includegraphics[width=1.5cm]{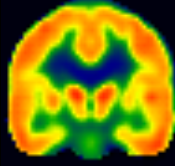}
		\end{subfigure}&
		
		\begin{subfigure}{1.5cm}
			\centering\includegraphics[width=1.5cm]{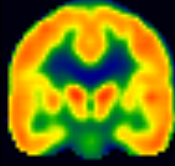}
		\end{subfigure}&
		\begin{subfigure}{1.5cm}
			\centering\includegraphics[width=1.5cm]{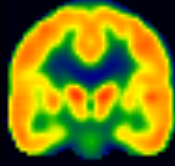}
		\end{subfigure}&
		\begin{subfigure}{1.5cm}
			\centering\includegraphics[width=1.5cm]{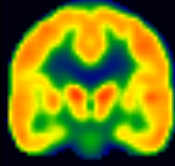}
		\end{subfigure}\\

		%%%%%%%%%%%%%%  c
		&
		\begin{subfigure}{1.5cm}
			\centering\includegraphics[width=1.5cm]{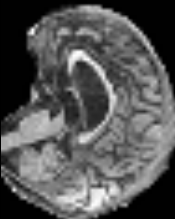}
		\end{subfigure} &
		\begin{subfigure}{1.5cm}
			\centering\includegraphics[width=1.5cm]{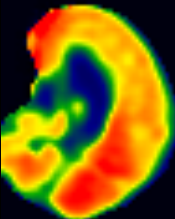}
		\end{subfigure}&
		\begin{subfigure}{1.5cm}
			\centering\includegraphics[width=1.5cm]{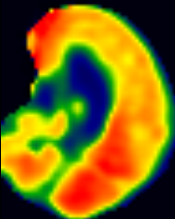}
		\end{subfigure}&
		\begin{subfigure}{1.5cm}
			\centering\includegraphics[width=1.5cm]{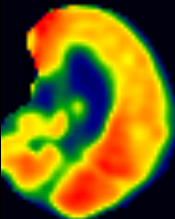}
		\end{subfigure}&
		
		\begin{subfigure}{1.5cm}
			\centering\includegraphics[width=1.5cm]{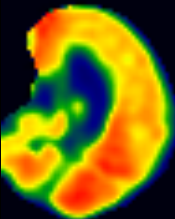}
		\end{subfigure}&
		\begin{subfigure}{1.5cm}
			\centering\includegraphics[width=1.5cm]{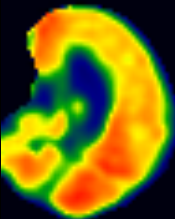}
		\end{subfigure}&
		\begin{subfigure}{1.5cm}
			\centering\includegraphics[width=1.5cm]{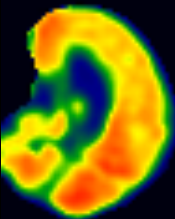}
		\end{subfigure}\\
		
	\end{tabular}

	\caption{\label{fig:cond_samples} Age information manipulation. There are 3 subjects, AD, MCI, and CN, each subject provides $6$ results \textit{w.r.t.} a variant of age labels.}
\end{figure*}

\begin{figure*}[h]
	\centering
	\includegraphics[width=.8\textwidth]{./figs/cond_quan.eps}
	\vspace{-4mm}
	\caption{\label{fig:cond_quan} The mean intensity of $12$ ROIs with the change of age for $3$ average subjects.}
\end{figure*}

\subsection{\label{sec: quality}Evaluation of Generated vs. Ground Truth Images}

We begin our model evaluation by comparing outputs from our model to a baseline method used previously for similar image generation tasks, 3D-GANs (Generative Adversarial Networks). We compare using commonly-used quantitative measures computed over the held out testing data. These include Mean Absolute Error (MAE), Correlation Coefficients (Cor\_Coef), Peak Signal-to-Noise Ratio (PSNR), and Structure Similarity Index (SSIM). For Cor\_Coef, PSNR and SSIM, higher values indicate better generation of PET images.  For MAE, the lower the value, the better the generation. There are six 3D convolutional layers in the generator of the 3D-GAN while the discriminator is a 3D CNN with 4 convolutional layers and 1 fully-connected layer. As seen in Table \ref{etb1}, our model competes favorably against the 3D-GAN.
\begin{table*}[h]
	%\vspace{-7mm}
	\begin{center}
		\caption{\label{etb1} Comparison of our method against the 3D-GAN baseline across four different reconstruction metrics.}
		\begin{tabular}{|c | c |   c| c |c|}
			\hline
			\footnotesize{METHOD}     & MAE    &CorCoef  &PSNR &SSIM \\
			\hline                                                  
			3D-GANs               &$ 0.0229\pm0.0396$
			&   $0.9583$ & $27.49\pm2.0857$ &  $0.7678\pm0.0746$
			\\
			\hline 
			\textbf{DUAL-GLOWs}    &$ \bm{0.0231} \pm \bm{0.0289}$
			&   $\bm{0.9754}$ & $\bm{29.56} \pm \bm{2.6622}$ &  $\bm{0.8978} \pm \bm{0.0615}$
			\\
			\hline
		\end{tabular}
	\end{center}
	%\vspace{-5mm}
\end{table*}
Standardized uptick value ratio (SUVR) is a ratio of radioactivity concentration specifically designed for evaluation of PET images. In this case, we directly compute the ratio of our generated image (GD) to that of the ground truth image (GT):
\begin{equation}
SUVR=\frac{SUV_{GT}}{SUV_{GD}} = \frac{\bar{i}_{GT}}{\bar{i}_{GD}}.
\end{equation}
We compute this measure on 16 gray matter regions of interest\footnote{The 16 regions include bilateral Angular, Anterior Cingulum, Posterior Cingulum, Frontal Medial Gyrus Orbital, Precuneus, Supramarginal Gyrus, Middle Temporal Gyrus, and Superior Temporal Gyrus.
	%Angular\_L, Angular\_R, Cingulum\_Ant\_L, Cingulum\_Ant\_R, Cingulum\_Post\_L, Cingulum\_Post\_R, Frontal\_Med\_Orb\_L, Frontal\_Med\_Orb\_R, Precuneus\_L, Precuneus\_R, SupraMarginal\_L, SupraMarginal\_R, Temporal\_Mid\_L, Temporal\_Mid\_R, Temporal\_Sup\_L, Temporal\_Sup\_R} (ROIs) known be associated with developing AD pathology
	These regions have previously been identified as being associated with developing AD pathology \cite{kim2016adaptive}.
% \textit{Angular\_L, Angular\_R, Cingulum\_Ant\_L, Cingulum\_Ant\_R, Cingulum\_Post\_L, Cingulum\_Post\_R, Frontal\_Med\_Orb\_L, Frontal\_Med\_Orb\_R, Precuneus\_L, Precuneus\_R, SupraMarginal\_L, SupraMarginal\_R, Temporal\_Mid\_L, Temporal\_Mid\_R, Temporal\_Sup\_L, Temporal\_Sup\_R}.
}
These regions are first segmented based on the Automated Anatomical Labeling (AAL) atlas \cite{tzourio2002automated,rolls2015implementation}, and the SUVR is averaged over all image voxels within those regions. An SUVR closer to $1$ indicates better generation. Here, we use the relative SUVR ($rSUVR = |SUVR-1|$) for easier interpretation. As illustrated in Figure \ref{fig:suvr}, our model outperforms 3D GANs on most of the ROIs.

%\subsection{Quantitative Experiments}
A natural question may be that all generated 
images are the ``same", i.e.,
we are not inherently capturing any heterogeneity
within the cohort,
and are simply learning the average PET image
or a heavily skewed, cognitively normal PET image.
Figure \ref{fig:exp2} shows that this is not the case:
On the held out test set of samples,
the mean squared error between the generated 
and ground truth image is \textit{not}
correlated with age,
gender, or disease status.

Figures \ref{fig:samples-ad}, \ref{fig:samples-cn}, and \ref{fig:samples-mci} display test images generated after 90 epochs for Cognitively Normal, Mild Cognitive Impairment, and Alzheimer's Disease individuals.
Qualitatively, not only is the model able to accurately construct large scale structures
such as skull shape and grey matter density,
but it is also able to identify
minute, sharp boundaries between grey matter and white matter.
While here we focus on data
from individuals with a clear progression of
Alzheimer's disease from those who are clearly 
cognitively healthy, in preclinical cohorts
where disease signal may be weak, accurately constructing
finer-grained details may be critical
in identifying those at risk for developing dementia.

\subsection{Scientific Evaluation of Generation}

As evidenced above, the proposed method is able to 
learn the modality mapping from MRI to PET. 
However, often image acquisition is used as a means to an end:
typically towards disease diagnosis or informed preventative care.
While the generated images may seem computationally and visually coherent,
it is important that the images generated add some value towards these
downstream analyses. 

We construct simple t-tests to explore the consistency of diagnosis
between ground truth and generated images. For both sets of images,
we select AD positive and control normal (CN) individuals from 
the test set and compute the voxel-wise t-test between the two groups.
Using a standard $\alpha =0.05$ cutoff, we obtain binary masks indicating
regions of the brain showing a significant difference between healthy and
diseased individuals for both ground truth and generated images.
%We also do the t-test to explore the consistence between ground truth and synthetic PET images in the anatomic analysis of AD. We select the AD and CN subjects in testing data and do the t-test for each voxel with the two groups.
%Given the cut-off $0.05$ of p-value, we obtain three binay mask, which show the specific region associated with AD.
As we can see from Figure \ref{fig:t-test},
there exist significant overlapping regions between the synthetic PET images and the ground truth ones in the testing data.
We expect that with more samples, consistency among disease-related regions will increase.

We also evaluate the generated PET images for the disease prediction and classification. Using the AAL atlas, we obtain all 116 ROIs via atlas-based segmentation \cite{wu2007optimum}. We select the mean intensity of all ROIs to be used for image features.
%Using support vector regression (SVR), we learn a model based on PET images in the training set to predict a continuous variable indicating disease status (0.0 for CN, 0.2 for SMC, and so on up to 1.0 for AD).
A support vector machine (SVM) is trained with the standard RBF kernel to predict binary disease status (Normal, EMCI, SMC vs. MCI, LMCI, AD) for both the the ground truth and the generated images. The SVM trained on generated images achieves comparable accuracy and false positive/negative rates (Table \ref{etb2}), suggest that the generated images contain sufficient signal in disease diagnosis.
%Finally, we calculate the classification accuracy on both the ground truth and generated images in the test set (Table \ref{etb2}). The SVM trained on generated images achieves comparable classification accuracy against the ground truth, indicating that for AD classification generated PET images can be used without significant loss.
%\textbf{false pos/false neg discuss here, also adding SVR results.}
% The qualitative result shows that our generated PET image can be seamlessly used for AD pathology analysis and study.

\begin{table*}[t]
	%\vspace{-7mm}
	\begin{center}
		\caption{\label{etb2}  Validation on the ground truth and synthetic images for the AD/CN classification.}
		\begin{tabular}{lC{3cm}  C{3cm} }
			\hline
			& Ground Truth    & Synthetic Images \\
			\hline                                                  
			Accuracy &$94\%$ & $91\%$\\
			False Negative Rate & $6\%$ & $6\%$ \\
			False Positive Rate & $0\%$ & $3\%$ \\
			\hline 
		\end{tabular}
	\end{center}
	%\vspace{-5mm}
\end{table*}

{\bf Conditional Framework for Side Information Manipulation.}
The conditional framework naturally allows us to evaluate potential developing pathology with age of the patient. Training the full model, we use ground truth side information (age) as the conditioning variable described above. Figure \ref{fig:cond_samples} shows the continuous change in the $3$ generated images given various age labels for the same MRI. The original image (left) is at the age of $50$, and as the age moves from $60$ to $100$ increased neuropathology becomes clear. To quantitively evaluate our conditional framework, we plot the mean intensity value of the $12$ ROIs. As demonstrated in Figure \ref{fig:cond_quan}, the mean intensity value changes smoothly across age, and as expected larger disease burden reflects a baseline shift across all ages.
